# Supplementary material for: Deterministic equivalent and error universality of deep random features learning
Source: arXiv:2302.00401 source file (2023-02-01)
Supplement: Supplementary file 1 [file anisotropic.tex]

Appendix for the proof of anisotropic deterministic equivalent.
